# Supplementary material for: Scaling up GANs for Text-to-Image Synthesis
Source: arXiv:2303.05511 source file (2023-06-19)
Supplement: Supplementary file 2 [file fid_clip_truncation.tex]

\begin{figure}[b]
    \centering
    \includegraphics[width=0.94\linewidth]{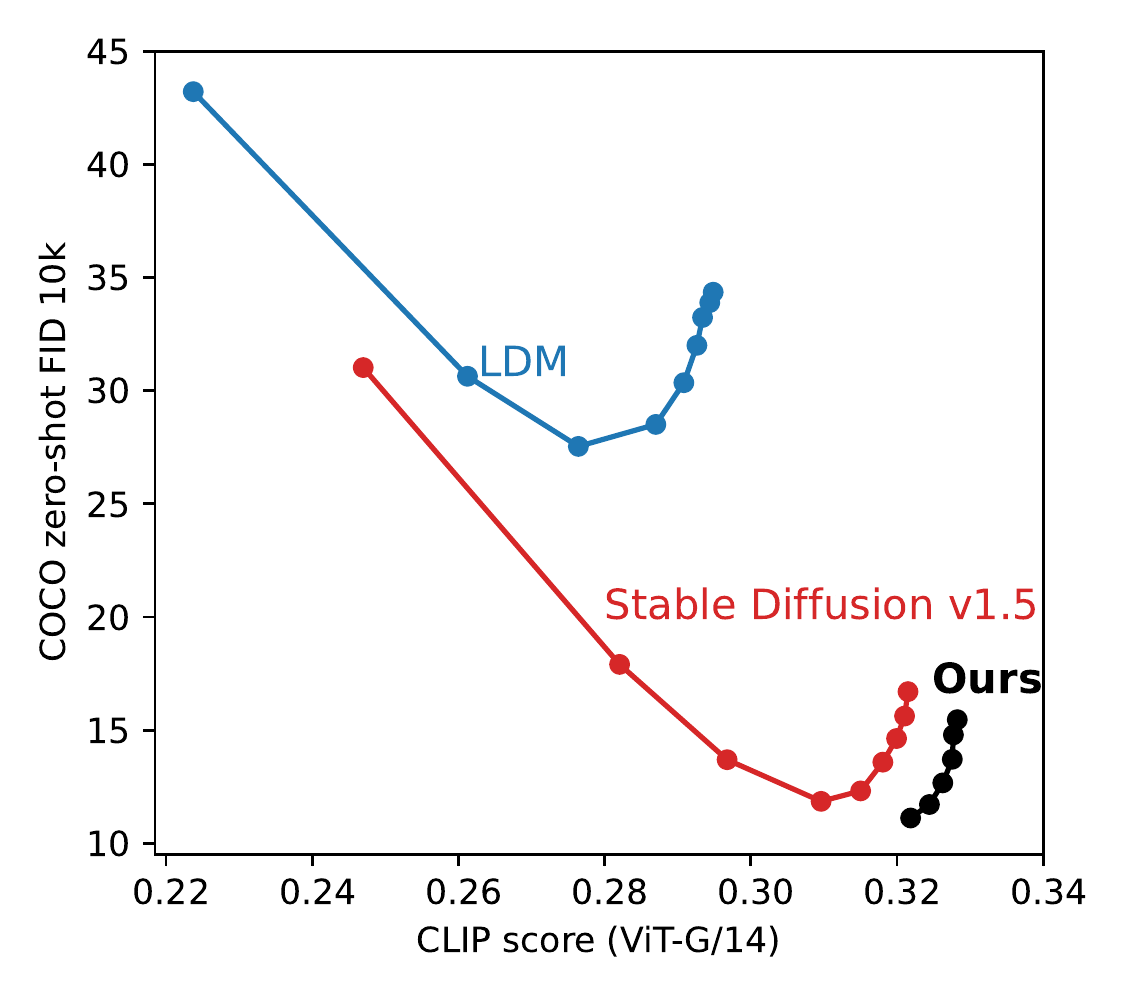}
    \vspace{-4mm}
    \caption{ We investigate how our FID and CLIP score changes over different truncation values [1.0, 0.9, 0.8, 0.7, 0.6, 0.5], by visualizing them along with the FID-CLIP score curve of two publicly available diffusion models: LDM and Stable Diffusion. The CLIP score increases with more truncation at the cost of reduced diversity indicated by higher FID. 
    }
    \label{fig:suppmat_truncation_plot}
\end{figure}
