# Supplementary material for: Scaling up GANs for Text-to-Image Synthesis
Source: arXiv:2303.05511 source file (2023-06-19)
Supplement: Supplementary file 3 [file 4_ImageNet_comparison.tex]

\input{Supplement/Figures/Imagenet1}
\input{Supplement/Figures/Imagenet2}
